# Supplementary material for: PAC Mode Estimation using PPR Martingale Confidence Sequences
Source: arXiv:2109.05047 source file (2022-04-11)
Supplement: Supplementary file 2 [file optimality_k_general.tex]

\section{Proof of Optimality for General K}

Let the $D(\mathcal{P}||\mathcal{P}')$ denote the divergence term in the Sequential Mode estimation paper for a distribution with K classes. Assume the true means are $p_1 > p_2 \geq \dots p_k $ Let $D(p||0.5)$ denote the term that arises in the lower bound for K=2, with the mode having a probability p. 

\subsection{Useful Lemmas}

\subsubsection{Lemma 1}

$$(p_1+p_2)D\left(\frac{p_1}{p_1+p_2} || 0.5\right) = D(\mathcal{P}||\mathcal{P}')$$

Proof,

\begin{align*}
    (p_1+p_2)D\left(\frac{p_1}{p_1+p_2} || 0.5\right) &= p_1\log\left(\frac{p_1/(p_1+p_2)}{0.5}\right) + p_2\log\left(\frac{p_2/(p_1+p_2)}{0.5}\right) \\
    &= p_1\log\left(\frac{p_1}{(p_1+p_2)/2}\right) + p_2\log\left(\frac{p_2}{(p_1+p_2)/2}\right) \\
    &= p_1\log\left(\frac{p_1}{q}\right) + p_2\log\left(\frac{p_2}{q}\right) \\
    &= D(\mathcal{P}||\mathcal{P}')
\end{align*}

\subsubsection{Lemma 2}

Consider the following function,
$$F(p) = p_1\log\left(\frac{p_1}{(p_1+p)/2}\right) + p\log\left(\frac{p}{(p_1+p)/2}\right)$$
where $p_1$ is a constant such that $p_1 \in (0,1]$ and $p \in [0,p_1)$
\begin{align*}
    F(p) &= p_1\log(p_1) + p\log(p) - (p_1 + p)\log((p_1 + p)/2) \\
         &= p_1\log(p_1) + p\log(p) - (p_1 + p)\log(p_1 + p) + (p_1 + p)\log(2) \\
    F'(p)&= 1 + \log(p) - 1 - \log(p_1 + p) + \log(2) \\
         &= \log\left(\frac{2p}{p_1 + p}\right) < 0 \quad \forall p \in [0,p_1)
\end{align*}
\subsubsection{Lemma 3}

$$(p_1+p_i)D\left(\frac{p_1}{p_1+p_i} || 0.5\right) \geq D(\mathcal{P}||\mathcal{P}') \quad \forall p_i \in [0, p_2]$$

Proof: From Lemma 1,

\begin{align*}
(p_1+p_i)D\left(\frac{p_1}{p_1+p_i} || 0.5\right) &= p_1\log\left(\frac{p_1}{(p_1+p_i)/2}\right) + p_i\log\left(\frac{p_i}{(p_1+p_i)/2}\right) \\
&\geq p_1\log\left(\frac{p_1}{(p_1+p_2)/2}\right) + p_2\log\left(\frac{p_2}{(p_1+p_2)/2}\right) \\
&= D(\mathcal{P}||\mathcal{P}')
\end{align*}

The second line follows from Lemma 2 and from the fact that $p_2 \geq p_i$

\subsection{Actual  Proof}

For a given distribution $\mathcal{P}$, there exists $N(\mathcal{P}, \epsilon_2)$ such that 
$$E_{\alpha_1} = \left(\forall t \geq N(\mathcal{P}, \epsilon_2),\forall i \in \{1,2\dots,k\}, p_i^t - \hat{p}_i^t \leq \frac{\epsilon_2}{2} \right)$$

and $\mathbb{P}(E_{\alpha_1}) \geq 1 - \alpha_1$ \\

\noindent
Now suppose for a given $\epsilon > 0$ the number of samples completed is,

$$t^* = \frac{(1+\epsilon_1)}{D(\mathcal{P},\mathcal{P}')}\log\left(\frac{K-1}{\delta}\right) + f(\mathcal{P}, \delta, \epsilon_1, \epsilon_2)$$

\noindent
On the event $E_{\alpha_1}$ and using Lemma 2, the number of samples of arms 1 and i is

\begin{align*}
s_1^t + s_i^t &\geq (p_1 + p_i - \epsilon_2)\left(\frac{(1+\epsilon_1)}{D(\mathcal{P},\mathcal{P}')}\log\left(\frac{K-1}{\delta}\right) + f(\mathcal{P}, \delta, \epsilon_1, \epsilon_2)\right) \\
&\geq \frac{(1+\epsilon_3)}{D(p_1/(p_1+p_i),0.5)}\log\left(\frac{K-1}{\delta}\right) + f'(\mathcal{P}, \delta, \epsilon_1, \epsilon_2)
\end{align*}

\noindent
We can make the function f' large enough so that $\forall i, \mathbb{P}(\neg term_i^{t^*}) \leq \frac{\alpha_2}{K-1}$ \\

\noindent
Therefore if PPR has not terminated at time $t^*$, we must have either $\neg E_{\alpha_1}$ or $\exists i, \neg term_i^{t^*}$. Using a simple union bound the probability of either of these two events is bounded by $\alpha_1 + (K-1)*\frac{\alpha_2}{K-1} = \alpha_1 + \alpha_2$. \\

\noindent
So we finally get the condition,
$$\mathbb{P} \left(\lim_{\delta\rightarrow0}\sup\frac{\tau}{\log(1/\delta)} \leq \frac{1+\epsilon}{D\left(\mathcal{P} || \mathcal{P'}\right)} \right) \geq 1 - \alpha_1 - \alpha_2$$
