# Supplementary material for: PAC Mode Estimation using PPR Martingale Confidence Sequences
Source: arXiv:2109.05047 source file (2022-04-11)
Supplement: Supplementary file 3 [file optimalty_k2.tex]

\section{Proof of Optimality for K = 2}

\subsection{Sufficient Condition for PPR-Bernoulli Termination}

Consider a problem instance $\mathcal{P}(p, v, 2)$ having parameters $p_1$ and $p_2 = 1 - p_1$. Let us count a sample of class $v_1$ as a "1" and that of class $v_2$ as a "0". Suppose we have made t samples in total and observed k 1s, we further define the empirical parameters $\hat{p}_1^t = \frac{k}{t}$ and $\hat{p}_2^t = \frac{t-k}{t} = 1 - \hat{p}_1^t$.

Accoriding to our stopping rule we can terminate when

\begin{align*}
\text{Beta}(0.5; k + 1, t - k + 1) &\leq \delta \\
\frac{(0.5)^k(0.5)^{t-k}(t+1)!}{(k)!(t-k)!}  &\leq \delta \\
(0.5)^k(0.5)^{t-k}(t+1)\binom{t}{k} &\leq \delta
\end{align*}

Writing the condition in this form allows us to use the following well known~\footnote{See, for example, \url{https://arxiv.org/pdf/1406.7872.pdf}.} inequality, with $\alpha = \frac{k}{t}$

\begin{equation*}
    \binom{t}{\alpha t} \leq 2^{tH_b(\alpha)}\,\, \text{where $t \in \mathbb{N}$ and $\alpha \in \left[0, \frac{1}{2}\right].$} 
\end{equation*}

The definition of binary entropy function $H_b$ for $p \in [0, 1]$ is: 
\begin{equation*}
    H_b(p) = 
    \begin{cases}
    0 & p \in \{0, 1\},\\
    -p\log_2p - (1 - p)\log_2(1 - p) & \text{otherwise.}\\
    \end{cases}
\end{equation*}

Thus we arrive at a sufficient condition for PPR-Bernoulli termination

\begin{align*}
    (0.5)^k(0.5)^{t-k}(t+1)2^{tH_b(\frac{k}{t})} &\leq \delta \\
    k\log(0.5) + (t-k)\log(0.5) + \log(t+1) + tH_b\left(\frac{k}{t}\right) &\leq \log(\delta) \\
    t\left(\frac{k}{t}\log(0.5) + \frac{(t-k)}{t}\log(0.5) - \frac{k}{t}\log\left(\frac{k}{t}\right) - \frac{(t-k)}{t}\log\left(\frac{(t-k)}{t}\right) \right) &\leq \log\left(\frac{\delta}{t+1}\right) \\
    t\left(\hat{p}_1^t\log(0.5) + (1-\hat{p}_1^t)\log(0.5) - \hat{p}_1^t\log\left(\hat{p}_1^t\right) - (1-\hat{p}_1^t)\log\left((1-\hat{p}_1^t)\right) \right) &\leq \log\left(\frac{\delta}{t+1}\right) \\
    t\left(\hat{p}\log\left(\frac{\hat{p}}{0.5}\right) + (1-\hat{p})\log\left(\frac{1-\hat{p}}{0.5}\right)\right) &\geq \log\left(\frac{t+1}{\delta}\right) \\   
    tD(\hat{p}_1^t||0.5)&\geq \log\left(\frac{t+1}{\delta}\right)
\end{align*}

\subsection{Asymptotic Bound for Samples Required under Sufficient Condition}

The arguments in this section are along the lines of those used for bandits \cite{JMLR:v17:kaufman16a}.

We fix $\epsilon$ and introduce,
$$\sigma = \max \left\{t \in \mathbb{N}^*, D\left(\hat{p}_1^t || 0.5\right) \leq  \frac{D\left(p_1 || 0.5\right)}{1 + \epsilon/2} \right\}$$

By the law of large numbers, $\mathbb{P}(\sigma < +\infty) = 1$. Hence, $\lim\limits_{n\rightarrow\infty} \mathbb{P}(\sigma \leq n) = 1$ and for every
$\alpha \in (0, 1)$ there exists $N(\epsilon, \alpha, p_1)$ such that $\mathbb{P}(\sigma \leq N(\epsilon, \alpha, p_1)) \geq 1 - \alpha$. Therefore,
introducing the event

$$E_\alpha = \left(\forall t \geq N(p, \epsilon, \alpha), D\left(\hat{p}_1^t || 0.5\right) >  \frac{D\left(p_1 || 0.5\right)}{1 + \epsilon/2}\right) \text{, one has } \mathbb{P}\left(E_\alpha\right) \geq 1 - \alpha $$

On the event $E_\alpha$,

\begin{align*}
\tau &\leq \max\left(N(\epsilon, \alpha, p_1), \inf \left\{ t \in \mathbb{N}: t\frac{D\left(p_1 || 0.5\right)}{1 + \epsilon/2} \geq \log\left(\frac{t+1}{\delta} \right)\right\}\right) \\
\tau &\leq N(\epsilon, \alpha, p_1) + \inf \left\{ t \in \mathbb{N}: t\frac{D\left(p_1 || 0.5\right)}{1 + \epsilon/2} \geq \log\left(\frac{t+1}{\delta} \right)\right\}
\end{align*}

Lemma 18 of Garivier et al. \cite{pmlr-v49-garivier16a} with $c_1 = \frac{D\left(p_1 || 0.5\right)}{1 + \epsilon/2}$, $c_2 = \frac{1}{\delta}$ and $\alpha = 1 + \gamma$ gives us the following bound

$$\tau \leq N(p, \epsilon, \alpha) + \frac{(1+\gamma)(1+\epsilon/2)}{D\left(\mathcal{P} || \mathcal{P'}\right)}\left(\log\left(\frac{e}{\delta}\left(\frac{1+\epsilon/2}{D\left(\mathcal{P} || \mathcal{P'}\right)}\right)^{1+\gamma} \right) + \log\left(\log\left(\frac{1}{\delta}\left(\frac{1+\epsilon/2}{D\left(\mathcal{P} || \mathcal{P'}\right)}\right)^{1+\gamma} \right)\right) \right)$$

We can make $\gamma$ small enough such that $(1+\gamma)(1+\epsilon/2) \leq (1 + \epsilon)$ and we have proved the condition

$$\mathbb{P} \left(\lim_{\delta\rightarrow0}\sup\frac{\tau}{\log(1/\delta)} \leq \frac{1+\epsilon}{D\left(\mathcal{P} || \mathcal{P'}\right)} \right) \geq 1 - \alpha$$
