# Supplementary material for: PAC Mode Estimation using PPR Martingale Confidence Sequences
Source: arXiv:2109.05047 source file (2022-04-11)
Supplement: Supplementary file 7 [file figures.tex]

\newpage

\section{RATIO OF OBSERVED SAMPLE COMPLEXITY TO LOWER BOUND}
\label{app:asymptotic-plot}

In this section we plot the ratio of our experimental sample complexity (averaged over 100 iterations) and the lower bound from Theorem~\ref{thm:lowerbound}~\citep{Shah_Choudhury_Karamchandani_Gopalan_2020} for values of $\delta$ ranging from $10^{-1}$ to $10^{-201}$. The distribution we consider is $\mathcal{P}_3$ from Table \ref{tab:tab_multiK}. We observe that KLSN-1v1 appears to be asymptotically optimal, along with PPR-1v1 (which we formally proved in Appendix~\ref{app:optimality-final}) while $\mathcal{A}_{1}$-1v1 seems suboptimal. We also observe that the 1v1 variant of each algorithm performs better asymptotically than its 1vr counterpart.
